# Supplementary material for: Concolic Testing for Deep Neural Networks
Source: arXiv:1805.00089 source file (2018-08-04)
Supplement: Supplementary file 1 [file appendix.tex]

\appendix

\subsection{Settings for Comparison with DeepXplore}
\label{app:DeepXplore}

\subsubsection{Parameter Settings}

\begin{itemize}
    \item DeepConcolic
    \begin{itemize}
        \item $L_\infty$-norm ball radius = 0.3
        \item $L_0$-norm upper bound = 100
    \end{itemize}
    \item DeepXplore
    \begin{itemize}
        \item transformation = `light', `occl', `blackout'
        \item weight\_diff = 1
        \item weight\_nc = 0.1
        \item step = 10
        \item seeds = 1
        \item grad\_iteration = 1000
        \item threshold = 0
        \item target\_model = 0 (our model)
        \item start\_point = (14, 14)
        \item occlusion\_size = (10, 10)
        \item constraint\_black(rect\_shape=(1, 1))
    \end{itemize}
\end{itemize}
Note that, as DeepXplore needs more than one DNNs, in this case we set our trained DNN as the target model, and utilise the other two default models in DeepXplore\footnote{\url{http://github.com/peikexin9/deepxplore}}.

\subsubsection{Platforms}
\begin{itemize}
 \item Hardware Platform:
    \begin{itemize}
        \item Intel(R) Core(TM) i5-4690S CPU @ 3.20\,GHz $ \times $ 4
    \end{itemize}
 \item Software Platform: 
    \begin{itemize}
        \item Fedora 26 (64-bit)
        \item Anaconda, PyCharm
    \end{itemize}
\end{itemize}

\subsection{Settings for Concolic Testing Results on Different Test Criteria}
\label{app:TestingResults}

\subsubsection{Model Architecture}
When evaluating the testing results of DeepConcolic, we train an MNIST DNN with architecture in Table~\ref{tbl:MNIST_Model}, and a CIFAR-10 DNN with architecture in Table~\ref{tbl:CIFAR10_Model}. 
\vspace*{3mm}
\begin{table}[h!]
	\caption{MNIST DNN architecture.}
	\label{tbl:MNIST_Model}
	\centering
	\vspace{2mm}
	\begin{tabular}{ l | c }
		\toprule
		Layer Type & MNIST \\
		\hline
		Convolution & 3 $\times$ 3 $\times$ 32 \\
		ReLU & \\
		Convolution & 3 $\times$ 3 $\times$ 32 \\ 
		ReLU & \\
		Max Pooling & 2 $\times$ 2 \\ 
		Convolution & 3 $\times$ 3 $\times$ 64 \\ 
		ReLU & \\
		Convolution & 3 $\times$ 3 $\times$ 64 \\ 
		ReLU & \\
		Max Pooling & 2 $\times$ 2 \\ 
		Flatten & \\ 
		Fully Connected & 200 \\ 
		ReLU & \\
		Fully Connected & 200 \\ 
		ReLU & \\
		Fully Connected & 10 \\ 
		Softmax & \\
		\bottomrule    
	\end{tabular}
\end{table}

\begin{table}[h!]
	\caption{CIFAR-10 DNN architecture.}
	\label{tbl:CIFAR10_Model}
	\centering
	\vspace{2mm}
	\begin{tabular}{ l | c }
		\toprule
		Layer Type & CIFAR-10 \\
		\hline
		Convolution & 3 $\times$ 3 $\times$ 32 \\
		ReLU & \\
		Convolution & 3 $\times$ 3 $\times$ 32 \\ 
		ReLU & \\
		Max Pooling & 2 $\times$ 2 \\ 
		Convolution & 3 $\times$ 3 $\times$ 64 \\ 
		ReLU & \\
		Convolution & 3 $\times$ 3 $\times$ 64 \\ 
		ReLU & \\
		Max Pooling & 2 $\times$ 2 \\ 
		Flatten & \\ 
		Fully Connected & 512 \\ 
		ReLU & \\
		Fully Connected & 10 \\ 
		Softmax & \\
		\bottomrule    
	\end{tabular}
\end{table}

\subsubsection{Platforms}
\begin{itemize}
 \item Hardware Platform:
    \begin{itemize}
        \item NVIDIA GeForce GTX TITAN Black
    \end{itemize}
 \item Software Platform: 
    \begin{itemize}
        \item Ubuntu 14.04.3 LTS
        \item Anaconda
    \end{itemize}
\end{itemize}
